# Supplementary material for: The Effect of Network Topology on Credit Network Throughput
Source: arXiv:2103.03288 source file (2021-09-28)
Supplement: Supplementary file 1 [file appendix-review-response.tex]

\newpage
\appendix
\noindent

\label{apdx:reviewer response}

\section{Response to SIGMETRICS 2021 reviews}
We thank the reviewers of ACM SIGMETRICS 2021 for their thoughtful and valuable comments comments. This section details the main concerns brought up by the reviewers and the changes we have made to address them. The \blue{colored} text describes our response, which contains pointers to the relevant parts of the paper that have been modified. 

Many reviewers brought up the practical relevance of this paper in influencing the design of real credit network topologies, particularly decentralized networks such as PCNs. 
\blue{We apologize for not mentioning this explicitly in the earlier version; however, even in decentralized networks like PCNs, system designers already exert real influence on network topology formation. For example, in the Lightning Network, an \emph{autopilot} system quickly bootstraps a new node and suggests potential peers for it to connect with. This recommendation uses node scores based on the number of channels a peer holds, the size of the channels, their longevity, and so on. Since nodes are incentivized via routing fees, 
new nodes have a vested interest in opening channels with peers in a manner that allows them to achieve high throughput without encountering deadlocks. We believe that these node scores can incorporate information based on the likelihood of deadlocks, and distance from an ideal deadlock-free topology to influence the creation of robust topologies in a decentralized manner.}

We respond to more specific concerns brought up by the reviewers below.

\subsection{Reviewer A}
\NewPara{What areas of the paper need improvement?}
\begin{itemize}
\item some assumptions and the methodology need more motivation and details, e.g., the flow assumptions for the evaluations. 

\blue{A couple of points: (1) Our evaluations also use the same discrete time model elaborated in \Sec{sec:model}, computing the maximum achievable (steady-state) throughput. The wording in \Sec{sec:eval-setup} and \Sec{sec:eval-metrics} has been clarified to specify that ``flows'' denote shortest paths between sender-receiver pairs that are allowed to move tokens in each epoch or discrete unit of time. The actual movement of tokens happens only over epochs. The word choice is solely to maintain consistency with \Sec{sec:topo peeling} where nodes on the left side of the bipartite graph are called \emph{flow nodes}, and not an alternate model. (2) Your point about ``heavy-hitters" among the nodes is valid. We have added detailed experiments in Appendix \ref{apdx:nonuniform random results} (mentioned in \Sec{sec:eval}), in which we consider nonuniform flow distributions, in which certain heavy-hitters participate in more flows than others. 
We observed similar trends to the uniform demand case, though these asymmetric demands require more flows to peel successfully, as you correctly predicted (more details below).
}

\item the connection between theoretical model and practical problem should be improved, also regarding relationship of throughput computations and topology design on the PCN operation. 

\blue{We have added text to \Sec{sec:intro} before our contributions and a remark at the end of \Sec{sec:eval-synthesis} that address the practical relevance of our study. As mentioned before, existing PCNs already have mechanisms in place to influence channel creation. Moreover, operators are individually incentivized to open channels  that support high throughput. Hence, we believe these observations can be leveraged to influence robust topology design. 
% Finally, as mentioned above, our theoretical model \Sec{sec:model} and the evaluations in \Sec{sec:eval} use the same model and metrics.
}
\end{itemize}

\NewPara{Comments for author(s)}.
%In general, the paper studies an interesting problem and the theoretical results, e.g., on the complexity and peeling, are sound. The writing quality and in particular the explanations of PCNs are good. 

%However, 
I am currently not convinced of the practical relevance of the study: 
\begin{itemize}
\item PCNs typically are decentralized by design, and it would be good to elaborate more on your assumption on the control: e.g., for topology design, why should the agents/nodes connect in the way that you describe? I understand that generalizing this might be planned for follow-up work, but at the moment it is not discussed at all and hence the practical connection is not as strong as it could be.

\blue{We recognize that it is hard to directly control the topology of decentralized networks. However, existing PCNs such as the Lightning Network, already use mechanisms to influence channel creation. In particular, an \emph{autopilot} system quickly bootstraps a new node and recommends peers based on the number of channels a peer holds, the size of the channels, their longevity, and so on. Since nodes reap routing fees for successful transactions, they are incentivized to open channels in a manner that allows them to achieve high throughput without encountering deadlocks. We believe that these node scores can incorporate information based on the likelihood of deadlocks, and distance from an ideal deadlock-free topology to influence the creation of robust topologies in a decentralized manner. We have added text to \Sec{sec:intro} before our contributions and a brief remark at the end of \Sec{sec:eval-synthesis} that address this.}

\item Regarding the evaluation methodology, you ``generate demand matrices with a fixed number of flows by sampling unique source-destination pairs at random from the set of nodes in the graph''. It would be good to elaborate on this model and its implications. I would have guessed that it would rather be the case that there are some ``large'' nodes, to which many users connect, in order to relay payments across the network? In your assumptions, all nodes are created ``equal'' with respect to the flows, thus having many easily peelable parts, but my feeling is that in reality, flows follow a very different distribution. I realize that getting data about this is not easy, but it would be good to have some discussion on the sensitivity of your results to this assumption, and what could be ``best case'' and ``worst case'' scenarios for your approach. 

\blue{We have included an evaluation with a skewed demand matrix where certain ``heavy-hitter'' nodes (10\% of all nodes) are more likely (70\% of the time) to be sampled as senders and receivers than the remaining nodes of the network. We compare the throughput behaviors of different topologies and understand how the \dpp in explains these behaviors in \App{apdx:nonuniform random results}. The overall trends across topologies are similar (\Fig{nonuniform random overall tpt}) and the evolution of the ripple during the \dpp is able to predict the relative performance of different topologies quite well (\Fig{nonuniform random peeling real evolution}). However, unlike the uniform random demand matrix, the LT code analysis based on the path length distribution alone does not predict the ripple evolution trajectory. This is not surprising: the LT code analysis assumes an i.i.d. bipartite graph wherein input symbols (channels) are chosen at random across flows (encoded symbols). It is rather fortunate that the uniform random demand case is close enough to this model that we can make simplifying assumptions and extend the LT codes analysis. However, with a skewed demand matrix, this analysis needs to be revisited to consider correlations. One approach is to condition the flow release probabilities on a channel degree distribution. We leave this analysis to future work, but believe that the rest of the synthesis pipeline can be adapted to use the revised analysis. We have acknowledged these differences both in \Sec{sec:eval-overall} and \App{apdx:nonuniform random results}.}

\end{itemize}


\subsection{Reviewer B}
\NewPara{What areas of the paper need improvement?}
\begin{itemize}
\item This paper assumes that transactions in the credit network occur synchronously over epochs, but not mention that in the evaluation part. 

\blue{We have clarified in \Sec{sec:eval-metrics} that we compute  the steady state per-epoch minimum and maximum throughput across all balance states. This is computed by solving the per-epoch LP specified in \Eqn{psi} at the center state of the balance polytope and the maximum-deadlock state, respectively.}

\item This paper only considers shortest-path algorithm for path selection and one path per transaction which is not realistic.

\blue{We have added a footnote in \Sec{sec:eval-setup} clarifying that additional edge-disjoint paths per demand pair and sampling more demand pairs have  similar effects on the path diversity in the network. They both add more paths to the network, albeit with slight differences in the number of shared nodes and edges. We use the latter approach for more control in our evaluations. We discuss this in more detail below in a similar comment's response.}
\end{itemize}

\NewPara{Comments for author(s)}.
\begin{itemize}
\item{In evaluation part, it's not clear whether the throughput is of one epoch. Are these flows all take place in one epoch or how many flows happen in one epoch? This paper assumes the balances of all channels remain unchanged after the epoch. But the question is a channel may actually not be able to support a transaction after some previous transactions in the same epoch, while the un-updated channel balance shows the enough capacity.}

\blue{We have clarified in \Sec{sec:eval-metrics} that in the evaluation, we compute  the steady state per-epoch minimum and maximum throughput across all balance states. This is computed by solving the per-epoch LP specified in \Eqn{psi} at the center state of the balance polytope and the maximum-deadlock state, respectively. The definitions of \ostpt $\psi$ (\Eqn{psi}) and $\maxtpt$ (\Eqn{phi}) are constrained by the definition of feasible flows (\Eqn{feasible flow}, \Eqn{feasible_flows}), which ensures that the total amount sent on a channel in a direction across all paths through it in a single epoch is less than the available balance at that end of the channel. This effectively means that all satisfying transactions can be supported simultaneously in that epoch. At the end of the epoch, the channel balance is updated to reflect the net amount that flowed on a channel in the two directions before this constraint is re-applied for the next epoch.}

\item Sometimes, the fact that a channel cannot support a transaction is not because the channel is used up in one direction. Mostly, it's because the channel doesn't have enough balances to support the flow, especially for large transactions. Dividing the transaction into several parts and finding path for each of them can somehow increase the success ratio. Or it can be simply routed through other channels. Actually, the throughput of shortest-path algorithm is much worse than many proposed routing algorithm such as Spider [NSDI'19], which can be taken into consideration. 

\blue{
Thank you for the comment; this is actually a subtle point. We would like to make two notes. 
First, we tried early in the project to vary the number of edge-disjoint shortest paths between a given demand pair, and compared the resulting min/max throughput to a setting with an equivalent number of total paths and total demand quantity, but each demand pair only had access to one shortest path for their transactions. 
Empirically, we found that these two settings give similar max and min throughput. 
This makes sense because our throughput LP assumes the presence of an ideal routing algorithm that can always achieve the maximum feasible amount on every permissible path in the routing matrix within the epoch. Though optimistic, this allows us to reason about throughput without concerning ourselves with the how exactly that throughput is achieved. In other words, we do not need to consider how the transaction is scheduled, whether it is split, and whether it is multiplexed in time or over paths the way Spider does.
We have added footnotes in \Sec{sec:eval-setup} and \Sec{sec:eval-metrics} that clarify this.
}

\blue{
Building on this point, we have also added a note re: \Fig{tpt sensitivity} (above Def.~\ref{def:worst_tpt}) that a better routing algorithm cannot mitigate or avoid the deadlock, but might be able to delay it. In fact, the Spider [NSDI'20] paper also discusses the phenomenon of reduction in circulation throughput due to DAG demands in Fig.13 of their paper.}
\end{itemize}

\subsection{Reviewer C}
\NewPara{What areas of the paper need improvement?}
\begin{itemize}
    \item The notions of min/max throughput and deadlock rely on best and worst-case flow assumptions, which might both be far away from reality in practical scenarios.
    
    \blue{When defining \wctpt (Def.~\ref{def:worst_tpt}), we have clarified that we capture the sensitivity of a topology using its best- and worst-case throughput behaviors because it is difficult to obtain information on the likelihood of observing different balance states in a \cn. This is because channel balances, particularly in PCNs, are only known to the end-points. It is therefore hard to argue that a topology with a large deadlock is ``unlikely" to occur; (a) not only do we not have access to typical transaction patterns, \emph{nobody does by design}, and (b) transient demand fluctuations, which cause these networks to end up in bad states, 
    are even harder to characterize than long-term patterns. For this reason, we study the worst throughput that a topology can achieve, given a certain model of the demand, across all of its balance states.}

    \item It is unclear how insights on deadlock properties of some common network models can inform the design of real credit networks
    
    \blue{We have also added text to \Sec{sec:intro} before our contributions and remarks at the end of \Sec{sec:eval-synthesis} that address the practical relevance of such a study. In particular, existing PCNs already have mechanisms in place to influence channel creation and are incentivized to open channels in a way that supports high throughput. We believe we can leverage both these aspects to influence robust topology design.}
\end{itemize}

\NewPara{Comments for author(s)}.
\begin{itemize}
\item 
%The paper does a really nice job formalizing the problem and defining notions of maximum and minimum throughput and of deadlocked channels, and shows some important fundamental relationships between these notions. At the same time, 
The focus of \Sec{sec:worst tpt} is a worst-case analysis, and seems somewhat artificial: In particular, it only considers circular flows, while there is no reason in general to assume that there is no "one-way" component in transaction demand. 

\blue{We have added clarifications in \Sec{sec:metrics} just before Def.~\ref{def:psi} that discusses that our demand is not restricted to just circulation flows. In fact, we are interested in demands that are a mix of circulation and DAGs (one-way transactions) and the impact that DAG demands have on the long-term (circulation) throughput of the credit network. We assume that rebalancing does not occur and instead focus on irrevocable loss of throughput due to perturbations in balance state caused by DAG demands. While our model does not assume circulations, the constraint that the state be unchanged at the end of an epoch in our definition of steady-state throughput ensures that our throughput LP only outputs circulation values (\Eqn{phi}).}

\item Also, while asking which topologies are more or less prone to deadlock is a fascinating question, in reality there is any control over the network formation process. On the contrary, the whole idea of peer-to-peer credit networks is that there is no centralized coordination.

\blue{We recognize that it is hard to directly control the topology of decentralized networks. However, existing PCNs such as the Lightning Network, already use mechanisms to influence channel creation. In particular, an \emph{autopilot} system quickly bootstraps a new node and recommends peers based on the number of channels a peer holds, the size of the channels, their longevity, and so on. Since nodes reap routing fees for successful transactions, they are incentivized to open channels in a manner that allows them to achieve high throughput without encountering deadlocks. We believe that these node scores can incorporate information based on the likelihood of deadlocks, and distance from an ideal deadlock-free topology to influence the creation of robust topologies in a decentralized manner. We have added text to \Sec{sec:intro} before our contributions and remarks at the end of \Sec{sec:eval-synthesis} that address this.}

\item Network topologies: The BA (pref-attachment) topology generates very peculiar networks with skewed degree distributions; as has been shown in the literature (eg [Doyle, Willinger, et al]), real-world ``scale-free'' networks tend to be very different, and conclusions from BA topologies don't necessarily carry over --> it would be helpful to try other power-law degree graphs to see if the observations are robust, or specific to BA.

\blue{We have added a comparison point with graphs with a power-law degree distribution to Figures.~\ref{fig:overall tpt comparison}, ~\ref{fig:peeling real evolution} and ~\ref{fig:peeling predicted evolution}. The general trends are similar to those of BA \sftopo graphs and the \lntopo. However, there are some behaviors such as a very long tail on the number of channels unpeeled as the number of demands is increased, that do not occur with BA or LN topologies. This in turn, affects the throughput behavior of the \pltopo topologies.}

\item I wonder if there would be more meaningful performance criteria that could have been studied. Ultimately, the goal of the network is to sustain transactions, while making ``rebalancing'' operations as rare as possible, given that these are costly. Under this point of view, the impact of deadlocks is temporary and limited. How would the insights on network topologies change under such a cost, which penalizes rebalance operations but does not preclude them?

% \vls{Can someone read this?}
\blue{This is an interesting question. There are a few issues at play, but in a nutshell, the throughput degradation and the extent of deadlock in different balance states can be quite different even for the same topology as seen in \Fig{tpt sensitivity}. Consequently, the benefit from rebalancing will also vary considerably depending on the starting state, the difference from the best-case throughput, and the rebalancing policy. 
We ultimately decided to remove this variable from our current study to avoid confounding factors.

That being said, it is not necessarily the case that rebalancing renders this whole discussion useless. 
For example, consider the effect of deadlock size, which is a function of the network's current state.
A small deadlock causes small throughput degradation, but the throughput can be restored using a coordinated operation between a small number of channels. However, large deadlocks, though rarer than small deadlocks, impact throughput significantly and make it harder to restore  throughput via coordinated efforts among many channels.
In fact, in Figure \ref{fig:peeling alg ilp comparison}, we see that even on small topologies, depending on the number of flows, we can end up with deadlocks of hundreds of edges, which may be difficult to resolve in a distributed fashion (unless the rebalancing policy is very aggressive, which leads to high rebalancing costs). 
This introduces the role of rebalancing strategy, which poses a complex new tradeoff between resources spent on rebalancing vs. total throughput. 

The second issue is that we simply don't have meaningful data about what network states or transaction patterns are typical (by design).
For these reasons, we capture the sensitivity of a topology using its best- and worst-case throughput behaviors. 
%Given that we lack data on the distribution of balanced states in a \cn and consequently, on what size deadlocks are commonly observed, we focus on the scenario without rebalancing in an effort to understand the absolute worst-case behavior of a topology. 
% and have left further exploration of the role of rebalancing policies to future work.

}

\item I did not understand the caption of \Fig{peeling alg ilp comparison} $\rightarrow$ what lines and points are they referring to?

\blue{We apologize that this figure was not clear the first time around. We have added a clarification to this effect, but \Fig{peeling alg ilp comparison}'s lines are generated based on the number of channels unpeeled in each topology. Point in the same figure laid atop these lines correspond to the actual number of deadlocked channels. Since all points fall on the line, the two numbers match exactly.}
\end{itemize}
